# Supplementary material for: Real-Time Video Deblurring via Lightweight Motion Compensation
Source: arXiv:2205.12634 source file (2022-09-13)
Supplement: Supplementary file 1 [file tbl_l_motion.tex]

\begin{table}[t]
\centering
\aboverulesep = 0.4mm %
\belowrulesep = 0.4mm %
\setlength\tabcolsep{0pt}
\scalebox{0.90}{%
    \begin{tabularx}{1.11111\columnwidth}{
    Y
    >{\centering}p{0.171\columnwidth}
    >{\centering}p{0.171\columnwidth}
    >{\centering}p{0.171\columnwidth}
    >{\centering\arraybackslash}p{0.171\columnwidth}
    }
    \toprule
    \multirow{2}{*}{\makecell{Model}}& \multicolumn{2}{c}{Deblurring} & \multicolumn{2}{c}{Motion Compensation} \\
    % \cmidrule{1-2}
    \cmidrule(l){2-5}
    & PSNR & SSIM & PSNR & SSIM \\
    \midrule
    w/o $L_{motion}$ &   30.22 & 0.921 & 24.94 & 0.871 \\
    \rowcolor{lightlightgray} w/ $L_{motion}$  & 30.26 & 0.921 & 26.20 & 0.891 \\
    \midrule[0.01mm]
    % \midrule[0.01mm]
    \bottomrule
    \end{tabularx}%
}
% \caption{\change{Ablation study on our model with $L_{motion}$ and the motion layer. The model trained with both $L_{motion}$ and motion layer is our final model, the same final model reported in the last row of Table 2 in the main paper.}}
\caption{\change{Comparison of two models with and without $L_{motion}$}}
\label{tbl:l_motion}
\end{table}
